# Supplementary material for: Dynamical Spectra of Spin Supersolid States in Triangular Antiferromagnets
Source: arXiv:2404.14163 source file (2024-04-22)
Supplement: Supplementary file 1 [file Supersolid_SM.pdf]

# *Supplementary material*

# Dynamical Spectra of Spin Supersolid States in Triangular Antiferromagnets

Runze Chi,[1,2] Jiahang Hu,[1,2] Hai-Jun Liao,[1,3,*] and T. Xiang[1,2,4,†]

[1]*Beijing National Laboratory for Condensed Matter Physics and Institute of Physics, Chinese Academy of Sciences, Beijing 100190, China.*
[2]*School of Physical Sciences, University of Chinese Academy of Sciences, Beijing 100049, China.*
[3]*Songshan Lake Materials Laboratory, Dongguan, Guangdong 523808, China.*
[4]*Beijing Academy of Quantum Information Sciences, Beijing, China.*

## I. TENSOR NETWORK METHOD

In this study, we employ the same infinite projected entangled-pair state (iPEPS) as Ref. [R1] to represent the ground state

$|0\rangle =$ 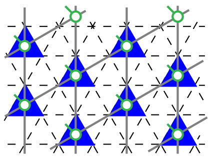 $=$ 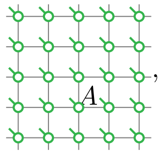, (Q1)



where we group three sites on a triangle into one site, making the original triangular lattice to a deformed square lattice. Each local tensor $A$ is composed of one physical index of dimension $d = 8$ and four virtual indices of dimension $D$, which controls the accuracy of the calculation. The local tensor $A$ can be determined by variational minimization of the ground state energy via automatic differentiation techniques [R2]. This wave function representation is compatible with all ground states of the easy-axis triangular-lattice antiferromagnetic XXZ model with a magnetic field, including the Y-shape, V-shape, up-up-down and fully polarized states.

To calculate spectral function, we construct a set of excited states $|\Phi_{\boldsymbol{k}}(B_m)\rangle$ with a definite momentum $k$ [R1, R3–R6], which are orthogonal to the ground state by replacing a local tensor $A$ at site $\boldsymbol{r}$ of the ground state $|\Psi(A)\rangle$ with a new tensor $B_m$ shown as follows

$$|m\rangle \equiv |\Phi_{\boldsymbol{k}}(B_m)\rangle = \sum_{\boldsymbol{r}} e^{i\boldsymbol{k}\cdot\boldsymbol{r}}$$ 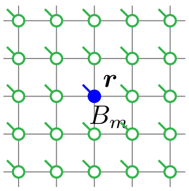 . (Q2)



Then, we compute the effective Hamiltonian $H^{\text{eff}}_{mn} = \langle\Phi_{\boldsymbol{k}}(B_m)|H|\Phi_{\boldsymbol{k}}(B_n)\rangle$ and the overlap matrix $N_{mn} = \langle\Phi_{\boldsymbol{k}}(B_m)|\Phi_{\boldsymbol{k}}(B_n)\rangle$ in this set of excited-state basis, and solve their generalized eigen-equation to obtain the excited energies $\{E_m\}$ and wavefunctions $\{|m\rangle\}$. Finally, we can obtain the zero-temperature dynamical spectral function

$$S^{\alpha\beta}(\boldsymbol{k},\omega) = \sum_m \langle 0|S^{\alpha}_{-\boldsymbol{k}}|m\rangle\langle m|S^{\beta}_{\boldsymbol{k}}|0\rangle\delta(\omega - E_m + E_0). \quad \text{(Q3)}$$

This method has been demonstrated to accurately obtain excitation spectra of frustrated magnetic systems [R1, R4–R7]. Here, we also benchmark the excitation spectra of fully polarized phases as shown in Fig. S1, and observe perfect agreement with the results from linear spin wave theory [R8], which is the exact solution for a fully polarized state because the fully polarized state does not involve quantum fluctuations. All our calculations were carried out using bond dimension $D = 4$ and Lorentz broading factor $\eta = 0.004$ meV if not specified otherwise.

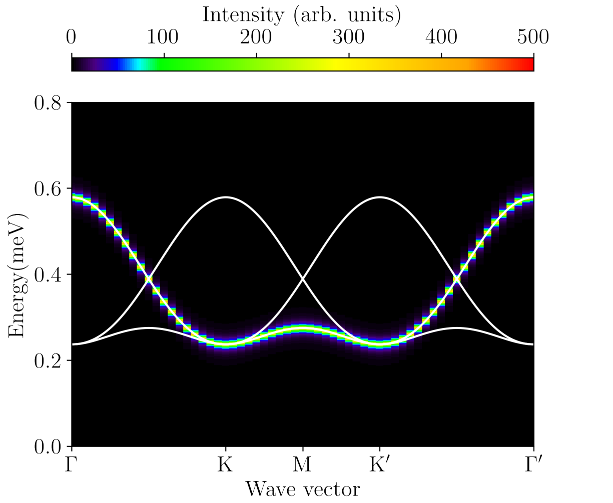


FIG. S1. The spectral function of the fully polarized state at magnetic field $B = 2.7$ T. The white lines denote the LSWT results. The tensor network results (solid squares) are obtained with bond dimension $D = 4$.

## II. BOND DIMENSION DEPENDENCE OF THE TWO LOWEST ENERGY GAPS

The antiferromagnetic XXZ model has a continuous U(1) symmetry, and should have a gapless Goldstone mode according to the Goldstone theorem. The reason why the lowest-energy branch in our results has a finite gap at the K point

* navyphysics@iphy.ac.cn
† txiang@iphy.ac.cn

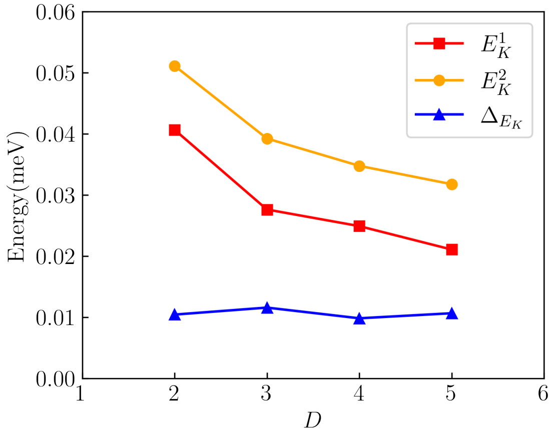


FIG. S2. The lowest and second lowest energy excited gaps at the K point as a function of the bond dimension $D$ of iPEPS.

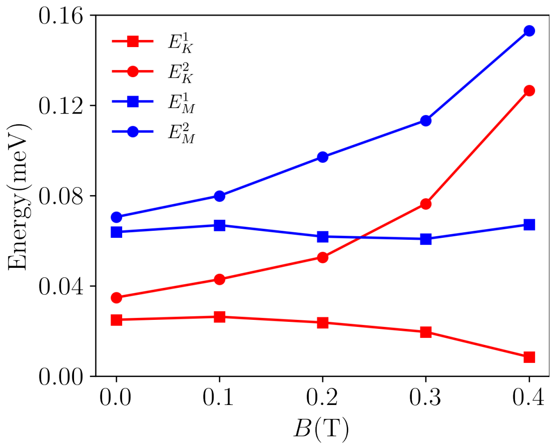


FIG. S3. The lowest (solid squares) and second lowest (solid circles) energy excited gaps at the K (red) and M (blue) points as a function of the magnetic field, respectively.

is because the tensor network method introduces a truncation parameter, the bond dimension $D$, which leads to a finite correlation length of ground state. Therefore, the excitation is always gapped when the bond dimension $D$ is finite, and becomes gapless only in the limit $D \to \infty$ (namely, $\xi \to \infty$). Practical computations [R1, R4–R7] have demonstrated that this gap induced by finite $D$ systematically decreases and gradually vanishes with increasing of $D$, thereby satisfying the Goldstone theorem. As shown in Fig. S2, our tensor network results indeed align with the expected outcomes. Both low energy modes at K point gradually decrease with the increasing of bond dimension $D$. More importantly, they consistently maintain a nearly constant energy spacing of about 0.01 meV (see the blue curve in Fig. S2), indicating that the second branch $E^2_{\mathrm{K}}$ should have an intrinsic finite gap of about 0.01 meV in the limit $D \to \infty$.

## III. EVOLUTION OF EXCITATION SPECTRA IN THE Y-SHAPE PHASE WITH MAGNETIC FIELD

Figure S4 illustrates the behaviors of the excitation spectra in the Y-shape supersolid phase as a function of magnetic field, where, as shown in Fig. 2(a) of the main text, the system remains in the Y-shape supersolid state for magnetic fields ranging from 0 T to 0.42 T. To distinguish the contributions of different spin fluctuation channels, we also plot the spectral functions $S^{xx}$, $S^{yy}$, and $S^{zz}$. Since the magnetic order lies in the $xz$ plane, $S^{yy}$ mainly exhibits the out-of-plane transverse fluctuations, while $S^{zz}$ and $S^{xx}$ mainly represent the in-plane fluctuations. As shown in Fig. S4 (k-o), the lowest and third lowest energy branches are primarily influenced by the out-of-plane fluctuations, whereas the second-lowest energy branch arises from the in-plane fluctuations, including the contributions from both the $S^{xx}$ and $S^{zz}$.

Furthermore, our tensor network results exhibit significant downward renormalization of magnons compared to the results of linear spin wave theory (the white lines in Fig. S4 (a-e)). In particular, the emergence of roton minima at the M point suggests the significant contributions of strong quantum fluctuations. At zero field, the spectra display two nearly degenerate roton excitation modes around the M point. As the magnetic field increases, these modes are away from each other (see Fig. S3), with the roton excitation vanishing from the Goldstone mode branch, suggesting that the roton dip in this mode may just result from the energy-level repulsion imposed by the roton excitations in the second lowest branch. On the other hand, the second lowest energy magnon excitations gradually shift to higher energies with increasing magnetic field, but consistently maintain a roton minimum at the M point. Moreover, the in-plane spectral functions ($S^{xx}$ and $S^{zz}$) show substantial high-energy spectral weights in the same spin excitation channel where the low-energy roton excitations appear. This indicates the existence of strong hybridization between in-plane transverse and longitudinal fluctuations, suggesting that the second roton excitation may arise from the hybridization of in-plane transverse and longitudinal modes. This can be seen from Fig. S4 (f-j) and (p-t). As the magnetic field increases, the spin alignment gradually orients towards the $z$ direction, leading to a gradual weakening of the coupling between the in-plane transverse and longitudinal modes. Consequently, the depth of the roton minimum also gradually decreases.

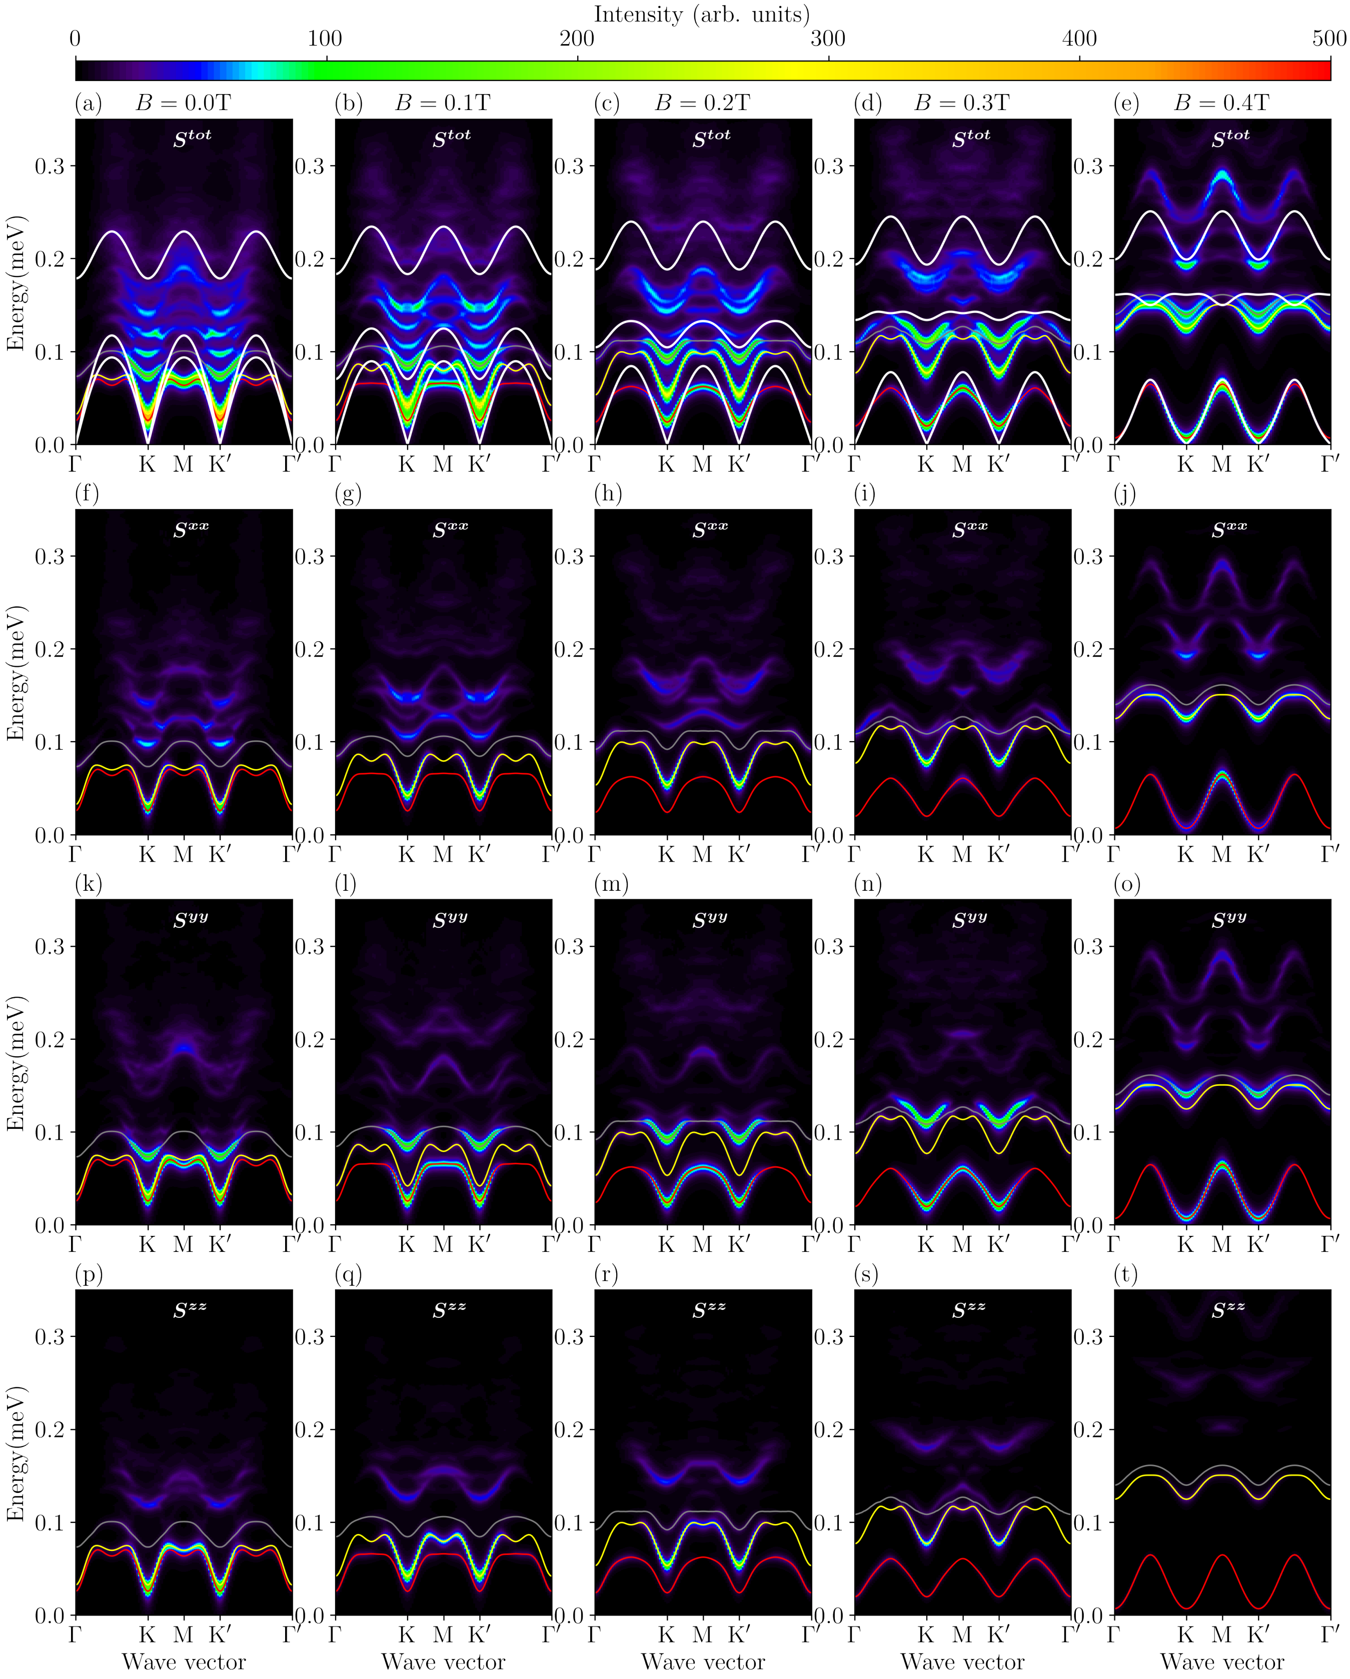


FIG. S4. The evolution of the dynamical spectral functions with magnetic field in the Y-shape phase. (a)-(e) The total spectral functions under magnetic fields of $B = 0.0, 0.1, 0.2, 0.3$ and $0.4$ T, respectively. The white curves denote the LSWT results. (f)-(j) The spin x-component spectral function. (k)-(o) The spin y-component spectral function. (p)-(t) The spin z-component spectral function.

[R1] R. Chi, Y. Liu, Y. Wan, H.-J. Liao, and T. Xiang, Phys. Rev. Lett. **129**, 227201 (2022).

[R2] H.-J. Liao, J.-G. Liu, L. Wang, and T. Xiang, Phys. Rev. X **9**, 031041 (2019).

[R3] L. Vanderstraeten, M. Mariën, F. Verstraete, and J. Haegeman, Phys. Rev. B **92**, 201111 (2015).

[R4] L. Vanderstraeten, J. Haegeman, and F. Verstraete, Phys. Rev. B **99**, 165121 (2019).

[R5] B. Ponsioen and P. Corboz, Phys. Rev. B **101**, 195109 (2020).

[R6] B. Ponsioen, F. F. Assaad, and P. Corboz, SciPost Phys. **12**, 006 (2022).

[R7] W.-L. Tu, L. Vanderstraeten, N. Schuch, H.-Y. Lee, N. Kawashima, and J.-Y. Chen, PRX Quantum **5**, 010335 (2024).

[R8] J. Sheng, L. Wang, W. Jiang, H. Ge, N. Zhao, T. Li, M. Kofu, D. Yu, W. Zhu, J.-W. Mei, Z. Wang, and L. Wu, (2024), arXiv:2402.07730 [cond-mat.str-el].
